# Supplementary material for: Bayesian Embeddings for Few-Shot Open World Recognition
Source: arXiv:2107.13682 source file (2022-10-06)
Supplement: Supplementary file 1 [file appendix.tex]

\subsection{Experimental Details}
\label{apx:exp}
